# Supplementary material for: Understanding the Ability of LLMs to Handle Character-Level Perturbation
Source: arXiv:2510.14365 source file (2026-05-28)
Supplement: Supplementary file 1 [file Similarity.tex]

\subsection{Feature Similarity w.r.t. Layer Index}
\begin{figure}[H]
    
\begin{tikzpicture}
\begin{axis}[
    xlabel={Layer},
    ylabel={Similarity},
    xmin=1, xmax=48,
    ymin=0.5, ymax=1,
    grid=both,
    grid style={line width=.1pt, draw=gray!30},
    major grid style={line width=.2pt,draw=gray!50},
    legend style={cells={anchor=west}, legend pos=north east},
    width=0.9\textwidth,
    height=8cm,
    cycle list name=exotic,  % 启用自动颜色分配
]

% 第一条折线
\addplot+[
    line width=1.5pt
] table[x=layer, y=similarity] {exp6_qwen330B_encoded=1.dat};
\addlegendentry{1}

\addplot+[
    line width=1.5pt
] table[x=layer, y=similarity] {exp6_qwen330B_encoded=2.dat};
\addlegendentry{2}

\addplot+[
    line width=1.5pt
] table[x=layer, y=similarity] {exp6_qwen330B_encoded=3.dat};
\addlegendentry{3}

\end{axis}
\end{tikzpicture}
\caption{Similairty of Hidden Features between Injection and Clean Text of Qwen3-30BA3B on GSM8K}
\label{fig:layers_similarity}
\end{figure}

\subsection{Feature Similarity w.r.t. Word Index in the Input}

\begin{figure}[ht]
    \centering
    \begin{tikzpicture}
    \begin{axis}[
        ylabel={Similarity},
        xlabel={Prefix word count},
        xmin=1, xmax=90,
        ymin=0.7, ymax=0.9,
        grid=both,
        grid style={line width=.1pt, draw=gray!30},
        major grid style={line width=.2pt,draw=gray!50},
        legend style={cells={anchor=west}, legend pos=north east},
        width=0.9\textwidth,
        height=8cm,
        cycle list name=exotic,
    ]
    \addplot[
        only marks,
        mark=*,
        mark size=1.5pt,
        red
    ] table {exp6_problem1.dat};
    \addplot[
        domain=0:90,
        thick,
        blue
    ] {-0.0006713588442688128*x+0.8275520033475642};
    \end{axis}
    \end{tikzpicture}
    %\vspace{\baselineskip} 
    \caption{Feature similarity between clean and noised inputs as noised tokens are progressively introduced during inference for a single input, evaluated with Qwen3-30B(A3B) non-thinking mode on the GSM8K problem 5 under \inj{1}.}
    \label{fig:similarity_token}
\end{figure}
